# Supplementary material for: Unveiling LLM Mechanisms Through Neural ODEs and Control Theory
Source: arXiv:2406.16985 source file (2025-02-23)
Supplement: Supplementary file 1 [file appendix.tex]

\section{Appendix A: Detailed Theoretical Proofs and Derivations in static analysis}

\subsection{Proof of Theorem 1}

\textbf{Theorem 1}: \emph{There exists a critical value \( \beta^* > 0 \) such that if \( \beta > \beta^* \), the market equilibrium results in one streamer capturing almost all viewers.}

\textbf{Proof}:

We aim to show that when the network effect parameter \( \beta \) exceeds a certain critical value \( \beta^* \), the equilibrium viewer distribution becomes highly concentrated, with one streamer capturing nearly all viewers.

Starting from the ratio of probabilities that a viewer chooses streamer \( i^* \) over any other streamer \( j \),Let \(\Delta q = q_{i^*} - q_j\) denote the difference in content quality between the top streamer \(i^*\) and another streamer \(j\). Then, the term becomes \(\alpha \Delta q\).
:

\[
\frac{P_{i^*}}{P_j} = \exp\left( \alpha \Delta q + \beta (n_{i^*} - n_j) \right)
\]

Since the total number of viewers is \( M \):

\[
n_{i^*} + (N - 1) n_j = M
\]

Express \( n_j \) in terms of \( n_{i^*} \):

\[
n_j = \frac{M - n_{i^*}}{N - 1}
\]

Substitute \( n_j \) back into the probability ratio:

\[
\frac{P_{i^*}}{P_j} = \exp\left( \alpha \Delta q + \beta \left( n_{i^*} - \frac{M - n_{i^*}}{N - 1} \right) \right)
\]

Simplify the expression:

\[
\frac{P_{i^*}}{P_j} = \exp\left( \alpha \Delta q + \beta \left( \frac{(N - 1) n_{i^*} - M + n_{i^*}}{N - 1} \right) \right) = \exp\left( \alpha \Delta q + \beta \left( \frac{N n_{i^*} - M}{N - 1} \right) \right)
\]

Assuming \( N \) is large, so \( N - 1 \approx N \), we have:

\[
\frac{P_{i^*}}{P_j} \approx \exp\left( \alpha \Delta q + \beta \left( n_{i^*} - \frac{M}{N} \right) \right)
\]

Now, the expected number of viewers for streamer \( i^* \) and \( j \) are:

\[
n_{i^*} = M P_{i^*}, \quad n_j = M P_j
\]

Therefore, the ratio of their viewer numbers is:

\[
\frac{n_{i^*}}{n_j} = \frac{M P_{i^*}}{M P_j} = \frac{P_{i^*}}{P_j} = \exp\left( \alpha \Delta q + \beta \left( n_{i^*} - n_j \right) \right)
\]

Substitute \( n_j \) with \( \frac{M - n_{i^*}}{N - 1} \):

\[
\frac{n_{i^*}}{\frac{M - n_{i^*}}{N - 1}} = \exp\left( \alpha \Delta q + \beta \left( n_{i^*} - \frac{M - n_{i^*}}{N - 1} \right) \right)
\]

Simplify the left-hand side:

\[
(N - 1) \frac{n_{i^*}}{M - n_{i^*}} = \exp\left( \alpha \Delta q + \beta \left( n_{i^*} - \frac{M - n_{i^*}}{N - 1} \right) \right)
\]

Again, for large \( N \), \( N - 1 \approx N \):

\[
N \cdot \frac{n_{i^*}}{M - n_{i^*}} = \exp\left( \alpha \Delta q + \beta \left( n_{i^*} - \frac{M - n_{i^*}}{N} \right) \right)
\]

Since \( \frac{M - n_{i^*}}{N} \) is small when \( n_{i^*} \) is close to \( M \), we approximate:

\[
N \cdot \frac{n_{i^*}}{M - n_{i^*}} \approx \exp\left( \alpha \Delta q + \beta n_{i^*} \right)
\]

Take natural logarithms on both sides:

\[
\ln N + \ln \left( \frac{n_{i^*}}{M - n_{i^*}} \right) = \alpha \Delta q + \beta n_{i^*}
\]

Assuming \( n_{i^*} \approx M - \epsilon \) with \( \epsilon \ll M \), we have:

\[
\frac{n_{i^*}}{M - n_{i^*}} = \frac{M - \epsilon}{\epsilon} \approx \frac{M}{\epsilon} - 1 \approx \frac{M}{\epsilon}
\]

Thus:

\[
\ln N + \ln \left( \frac{M}{\epsilon} \right) = \alpha \Delta q + \beta (M - \epsilon)
\]

Simplify the left-hand side:

\[
\ln N + \ln M - \ln \epsilon = \alpha \Delta q + \beta M - \beta \epsilon
\]

For large \( M \) and \( N \), \( \ln M \) and \( \ln N \) grow logarithmically, while \( \beta M \) grows linearly. Therefore, unless \( \beta \) is small, the right-hand side will dominate.

Rearranged:

\[
\beta M = \ln N + \ln M - \ln \epsilon - \alpha \Delta q + \beta \epsilon
\]

Since \( \epsilon \) is small, \( -\ln \epsilon \) is large and positive. For the equation to hold, \( \beta M \) must be sufficiently large, which implies a critical value \( \beta^* \).

Thus, there exists a critical \( \beta^* \) such that if \( \beta > \beta^* \), \( n_{i^*} \to M \), meaning streamer \( i^* \) captures almost all viewers, leading to the head effect.

\hfill\qedsymbol

\textbf{End of Proof}

\subsection{Proof of Theorem 2}

\textbf{Theorem 2}: \emph{Under the given parameters and assumptions, there exists a unique steady-state solution \( (n_i^*, q_i^*) \).}

\textbf{Proof}:

We consider the dynamic system where streamers adjust their content quality \( q_i \) to maximize profits, and viewers adjust their choices based on the utilities.

\textbf{Existence}:

- The set of possible viewer numbers \( n_i \) is bounded between 0 and \( M \), and the content quality \( q_i \) is bounded below (since producing zero quality is not profitable) and above (due to infinite costs at infinite quality).
- The best response functions derived from the streamers' optimization problem are continuous mappings from compact sets to themselves.
- By Brouwer's Fixed Point Theorem, a continuous function from a compact convex set to itself has at least one fixed point.
- Therefore, there exists at least one steady-state solution \( (n_i^*, q_i^*) \).

\textbf{Uniqueness}:

- The cost function \( c(q_i) \) is strictly convex (\( c''(q_i) > 0 \)), ensuring that the streamers' profit function is strictly concave in \( q_i \).
- The viewers' choice probabilities \( P_i \) are strictly increasing in \( \alpha_i q_i \) and \( n_i \), due to the properties of the multinomial logit model.
- The mapping from \( q_i \) to \( n_i \) is strictly increasing, and from \( n_i \) to \( q_i \) is strictly decreasing (since higher \( n_i \) implies streamers can reduce \( q_i \) for the same profit).
- The strict monotonicity ensures that the best response functions intersect at a unique point.
- Thus, the steady-state solution \( (n_i^*, q_i^*) \) is unique.

\hfill\qedsymbol

\textbf{End of Proof}

\subsection{Proof of Theorem 3}

\textbf{Theorem 3}: \emph{The steady state is locally asymptotically stable if all eigenvalues of the Jacobian matrix have negative real parts.}

\textbf{Proof}:

We analyze the dynamic system around the steady-state point \( (n_i^*, q_i^*) \) by linearizing the differential equations.

\textbf{Linearization}:

Let \( \delta n_i = n_i - n_i^* \) and \( \delta q_i = q_i - q_i^* \). The linearized system is:

\[
\frac{d}{dt} \begin{pmatrix} \delta n_i \\ \delta q_i \end{pmatrix} = J \begin{pmatrix} \delta n_i \\ \delta q_i \end{pmatrix}
\]

where \( J \) is the Jacobian matrix evaluated at the steady state.

\textbf{Jacobian Matrix}:

The Jacobian \( J \) consists of partial derivatives of the dynamic equations with respect to \( n_i \) and \( q_i \):

\[
J = \begin{pmatrix}
\frac{\partial \dot{n}_i}{\partial n_i} & \frac{\partial \dot{n}_i}{\partial q_i} \\
\frac{\partial \dot{q}_i}{\partial n_i} & \frac{\partial \dot{q}_i}{\partial q_i}
\end{pmatrix}
\]

Compute the partial derivatives:

1. \textbf{Partial Derivative of \( \dot{n}_i \)}:

\[
\frac{\partial \dot{n}_i}{\partial n_i} = \gamma \left( M \frac{\partial P_i}{\partial n_i} - 1 \right)
\]

2. \textbf{Partial Derivative of \( \dot{n}_i \) with respect to \( q_i \)}:

\[
\frac{\partial \dot{n}_i}{\partial q_i} = \gamma M \frac{\partial P_i}{\partial q_i}
\]

3. \textbf{Partial Derivatives of \( \dot{q}_i \)}:

From the streamer's optimization condition:

\[
c'(q_i) = (1 - \tau) R M P_i (1 - P_i) \alpha_i
\]

Differentiating both sides with respect to \( n_i \) and \( q_i \), we get:

\[
\frac{\partial \dot{q}_i}{\partial n_i} = - \frac{(1 - \tau) R M \alpha_i^2 P_i (1 - P_i) (1 - 2 P_i) \frac{\partial P_i}{\partial n_i}}{c''(q_i)}
\]

\[
\frac{\partial \dot{q}_i}{\partial q_i} = - \frac{(1 - \tau) R M \alpha_i^2 P_i (1 - P_i) (1 - 2 P_i) \frac{\partial P_i}{\partial q_i}}{c''(q_i)} - \frac{c'''(q_i)}{c''(q_i)} \dot{q}_i
\]

\textbf{Stability Condition}:

- The eigenvalues \( \lambda \) of \( J \) satisfy \( \det(J - \lambda I) = 0 \).
- If all eigenvalues have negative real parts (\( \text{Re}(\lambda) < 0 \)), the system returns to the steady state after small perturbations, indicating local asymptotic stability.
- The signs of the partial derivatives and the structure of \( J \) ensure that the eigenvalues have negative real parts under the given assumptions (e.g., \( \gamma > 0 \), \( c''(q_i) > 0 \), \( P_i (1 - P_i) > 0 \)).

\hfill\qedsymbol

\textbf{End of Proof}

\section{Appendix B: Theoretical Proofs in dynamic analysis}

\subsection{1. Existence and Uniqueness of Steady-State Solutions under the Dynamic Model}

\textbf{Theorem:} \emph{Under certain assumptions, the dynamic system has a unique steady-state solution \((n_i^*, q_i^*)\), where \(n_i^*\) is the steady-state number of viewers for streamer \(i\) and \(q_i^*\) is the steady-state content quality produced by streamer \(i\).}

\textbf{Proof:}

\textbf{Assumptions:}
\begin{itemize}
    \item \textbf{Continuity and Boundedness}: The functions involved in the dynamic equations are continuous and operate within bounded domains.
    \item \textbf{Strict Convexity}: The cost function \(c(q_i)\) is strictly convex and continuously differentiable in \(q_i\).
    \item \textbf{Monotonicity}: The response functions are monotonic with respect to their arguments.
    \item \textbf{Positive Parameters}: All parameters such as \(\alpha_i\), \(\beta\), \(\gamma\), \(M\), and \(R\) are positive.
\end{itemize}

\textbf{Dynamic Equations:}
\begin{itemize}
    \item Viewer Dynamics:
    \[
    \frac{d n_i(t)}{d t} = \gamma \left[ M P_i(t) - n_i(t) \right]
    \]
    where
    \[
    P_i(t) = \frac{\exp\left( V_i(t) \right)}{\sum_{k=1}^N \exp\left( V_k(t) \right)}
    \]
    and
    \[
    V_i(t) = \alpha_i q_i(t) - p_i + \beta n_i(t)
    \]

    \item Streamer Optimization:
    Streamers choose \(q_i(t)\) to maximize their profit:
    \[
    V_i(t) = (1 - \tau) R n_i(t) - c(q_i(t))
    \]
    The first-order condition (FOC) for maximization is:
    \[
    c'(q_i(t)) = (1 - \tau) R \frac{\partial n_i(t)}{\partial q_i(t)}
    \]
\end{itemize}

\textbf{Proof Steps:}
\begin{enumerate}
    \item \textbf{Existence of a Fixed Point}: Since the functions are continuous and the domain is compact (due to bounded \(n_i\) and \(q_i\)), Brouwer's Fixed Point Theorem guarantees the existence of at least one fixed point \((n_i^*, q_i^*)\).
    \item \textbf{Uniqueness of \(q_i^*\)}: From the FOC:
    \[
    c'(q_i^*) = (1 - \tau) R \frac{\partial n_i^*}{\partial q_i}
    \]
    The left-hand side (LHS) is strictly increasing in \(q_i^*\) due to the strict convexity of \(c(q_i)\). Therefore, there exists a unique \(q_i^*\) for each \(n_i^*\).
    \item \textbf{Uniqueness of \(n_i^*\)}: The steady-state equation \(n_i^* = M P_i^*\) can be shown to have a unique solution for \(n_i^*\) under the assumption that \(\beta\) is not too large, ensuring the mapping is a contraction.
\end{enumerate}

Thus, the steady-state solution \((n_i^*, q_i^*)\) is unique.

\subsection{2. Mathematical Theory and Proof of Path Dependence under the Dynamic Model}

\textbf{Theorem:} \emph{In the dynamic model with network effects, small differences in initial viewer numbers \(n_i(0)\) can lead to significant differences in long-term outcomes \(n_i^*\) due to path dependence, especially when the network effect parameter \(\beta\) is sufficiently large.}

\textbf{Proof:}

\textbf{Assumptions:}
\begin{itemize}
    \item \textbf{Positive Network Effects}: \(\beta > 0\).
    \item \textbf{Identical Streamers Except for Initial Viewers}: All streamers have identical parameters (\(\alpha_i = \alpha\), \(q_i(0) = q_0\), \(p_i = p\)), except for their initial viewer numbers \(n_i(0)\).
\end{itemize}

\textbf{Proof Steps:}
\begin{enumerate}
    \item The differential equation for viewer numbers:
    \[
    \frac{d n_i(t)}{d t} = \gamma \left[ M P_i(t) - n_i(t) \right]
    \]
    where
    \[
    P_i(t) = \frac{\exp\left( \alpha q_i(t) - p + \beta n_i(t) \right)}{\sum_{k=1}^N \exp\left( \alpha q_k(t) - p + \beta n_k(t) \right)}
    \]
    \item Consider two streamers \(i\) and \(j\) with initial viewer numbers \(n_i(0) > n_j(0)\). The initial difference \(\Delta n(0) = n_i(0) - n_j(0) > 0\) is amplified over time due to network effects, leading to a growing difference in their viewer numbers.
    \item The growth rate of the difference:
    \[
    \frac{d \Delta n(t)}{d t} = \gamma \left[ M (P_i(t) - P_j(t)) - \Delta n(t) \right]
    \]
    where \(P_i(t) > P_j(t)\), thus increasing the difference \(\Delta n(t)\) over time.
\end{enumerate}

As \(t \to \infty\), the viewer numbers for streamer \(i\) will dominate the system if \(n_i(0) > n_j(0)\) and \(\beta\) is large, leading to path dependence.

\subsection{3. Theoretical Proof of the Head Effect under the Dynamic Model}

\textbf{Theorem:} \emph{In the dynamic model with strong network effects (large \(\beta\)), the system exhibits the head effect, where one or a few streamers capture the majority of viewers, leading to significant market concentration.}

\textbf{Proof:}

\textbf{Assumptions:}
\begin{itemize}
    \item \textbf{Strong Network Effects}: The network effect parameter \(\beta\) is large.
    \item \textbf{Identical Streamer Characteristics}: All streamers have identical intrinsic attractiveness \(\alpha_i = \alpha\), pricing \(p_i = p\), and initial content quality \(q_i(0) = q_0\).
    \item \textbf{Small Initial Differences}: Small random variations exist in initial viewer numbers \(n_i(0)\) or content quality \(q_i(0)\).
\end{itemize}

\textbf{Proof Steps:}
\begin{enumerate}
    \item \textbf{Dynamics with Strong Network Effects}: The attractiveness \(V_i(t)\) of each streamer includes a term \(\beta n_i(t)\), which becomes dominant as \(\beta\) increases.
    \item \textbf{Amplification of Initial Differences}: Small initial differences in \(n_i(0)\) or \(q_i(0)\) lead to differences in \(V_i(0)\), affecting the choice probabilities \(P_i(0)\). With strong network effects, the term \(\beta n_i(t)\) significantly impacts \(P_i(t)\).
    \item \textbf{Positive Feedback Loop}: Streamers with slightly higher \(n_i(0)\) attract disproportionately more viewers due to higher \(P_i(t)\).
    \item \textbf{Market Concentration Metrics}: Define the market share \(s_i(t) = n_i(t)/M\), and the Herfindahl-Hirschman Index (HHI):
    \[
    \text{HHI}(t) = \sum_{i=1}^N s_i(t)^2
    \]
    As \(t \to \infty\), with strong network effects, \(s_i(t) \to 1\) for the dominant streamer(s), and \(s_j(t) \to 0\) for others, leading to \(\text{HHI}(t) \to 1\).
\end{enumerate}

This leads to the head effect, where one or a few streamers dominate the platform.

\section{AppendixB: Detailed Theoretical Proofs and Derivations}

\subsection{Proof of Welfare Impact Under the Head Effect}

\textbf{Proposition}: The head effect can lead to a decrease in total social welfare due to reduced consumer surplus from lack of diversity and a potential decrease in producer surplus as other streamers exit the market.

\subsubsection{Proof}

\begin{enumerate}
    \item \textbf{Consumer Surplus Impact}:
    
    - Under the head effect, \( n_{i^*} \approx M \) and \( n_j \approx 0 \) for \( j \neq i^* \).
    - Consumer surplus becomes:
    \[
    CS \approx M \left( \alpha q_{i^*} - p + \beta M \right)
    \]
    - While \( \beta M \) increases utility due to network effects, the lack of alternative content reduces the utility from variety. This loss of variety is not captured in the log-sum expression due to the dominance of \( i^* \).

    \item \textbf{Producer Surplus Impact}:
    
    - Total producer surplus is dominated by \( i^* \):
    \[
    PS \approx (1 - \tau) R M - c(q_{i^*})
    \]
    - Other streamers earn negligible profits, and some may exit the market, reducing content diversity and innovation.

    \item \textbf{Platform Profit}:
    
    - Short-term platform profit remains \( \Pi = \tau R M \), but long-term profit may decline if viewer engagement decreases due to lack of variety.

    \item \textbf{Social Welfare Comparison}:
    
    - Compare total welfare with and without the head effect. Without the head effect, more balanced \( n_i \) may lead to higher consumer surplus due to greater variety.
    - The exit of other streamers reduces producer surplus and overall social welfare.
\end{enumerate}

\textbf{Conclusion}: The head effect may reduce social welfare despite higher individual utility from network effects due to the negative impact on consumer surplus (from reduced variety) and producer surplus (from decreased competition).

\subsection{Derivation of Optimal Traffic Allocation Policy}

\textbf{Objective}: Maximize total social welfare \( W = CS + PS + \Pi \) with respect to \( \{ \theta_i \} \), subject to the constraints \( \theta_i \geq 0 \) and \( \sum_{i=1}^N \theta_i = 1 \).

\subsubsection{Lagrangian Formulation}

Define the Lagrangian function:
\[
\mathcal{L} = W - \lambda \left( \sum_{i=1}^N \theta_i - 1 \right) - \sum_{i=1}^N \mu_i \theta_i
\]
where \( \lambda \) is the Lagrange multiplier associated with the constraint \( \sum_{i=1}^N \theta_i = 1 \), and \( \mu_i \) are the Lagrange multipliers associated with the non-negativity constraints \( \theta_i \geq 0 \).

\subsubsection{First-Order Conditions}

For each \( \theta_i \), the first-order condition is:
\[
\frac{\partial \mathcal{L}}{\partial \theta_i} = \frac{\partial W}{\partial \theta_i} - \lambda - \mu_i = 0
\]

By complementary slackness, we have:
\[
\mu_i \theta_i = 0, \quad \mu_i \geq 0, \quad \theta_i \geq 0
\]

\subsubsection{Derivatives of Social Welfare}

\begin{enumerate}
    \item \textbf{Consumer Surplus Derivative}:  
    We assume that the change in the expected utility \(E[U_j]\) with respect to \(\theta_i\) is given by a factor \(1/\phi\). Hence,
    \[
    \frac{\partial CS}{\partial \theta_i} = M \frac{\partial E[U_j]}{\partial \theta_i} = M \frac{P_i}{\phi}.
    \]

    \item \textbf{Producer Surplus Derivative}:  
    \[
    \frac{\partial PS}{\partial \theta_i} = (1 - \tau) R \frac{\partial n_i}{\partial \theta_i}.
    \]

    \item \textbf{Platform Profit Derivative}:  
    \[
    \frac{\partial \Pi}{\partial \theta_i} = \tau R \frac{\partial n_i}{\partial \theta_i}.
    \]

    \item \textbf{Total Derivative of Viewer Numbers \( n_i \)}:  
    
    Using the properties of the multinomial logit model and incorporating the sensitivity factor \(\phi\), we have:
    \[
    \frac{\partial n_i}{\partial \theta_i} = M \frac{\partial P_i}{\partial \theta_i} = M P_i (1 - P_i) \phi.
    \]
\end{enumerate}

\subsubsection{Simplifying the First-Order Condition}

Combining the above derivatives, the first-order condition for welfare maximization is given by:
\[
M \frac{P_i}{\phi} + \left( (1 - \tau) R + \tau R \right) M P_i (1 - P_i) \phi = \lambda,
\]
where \(\lambda\) is the Lagrange multiplier. Simplifying, we obtain:
\[
\frac{P_i}{\phi} + R M P_i (1 - P_i) \phi = \lambda.
\]

\subsubsection{Case Analysis}

\begin{enumerate}
    \item \textbf{Interior Solution (\( \theta_i > 0 \))}:  
    For an interior solution, we have \(\mu_i = 0\), and the first-order condition simplifies to:
    \[
    M \left( \frac{P_i}{\phi} + R P_i (1 - P_i) \phi M \right) = \lambda.
    \]
    
    \item \textbf{Corner Solution (\( \theta_i = 0 \))}:  
    For a corner solution, where \(\theta_i = 0\) and \(\mu_i \geq 0\), the first-order condition becomes:
    \[
    M \left( \frac{P_i}{\phi} + R P_i (1 - P_i) \phi M \right) - \lambda \leq 0.
    \]
\end{enumerate}

\subsubsection{Conclusion}

The optimal traffic allocation \(\theta_i\) depends on the parameters \(P_i\), \(R\), \(M\), and the sensitivity factor \(\phi\). To maximize social welfare, the platform should allocate more traffic to streamers for which the marginal increase in social welfare per unit increase in \(\theta_i\) is the highest. In particular, streamers with lower \(P_i\) may contribute more to overall social welfare by enhancing diversity and increasing consumer surplus.

\subsection{Dynamic Optimization Problem}

In a dynamic context, the platform solves the following optimization problem to maximize the discounted sum of welfare over time:

\[
\max_{\{ \theta_i(t) \}} \int_0^\infty e^{-\rho t} W(t) \, dt
\]
subject to the dynamic equations for \( n_i(t) \) and \( q_i(t) \), and the constraints on \( \theta_i(t) \).

Where \( \rho \) is the discount rate.

\subsubsection{Hamiltonian Function}

Define the current-value Hamiltonian \( \mathcal{H} \):
\[
\mathcal{H} = W(t) + \sum_{i=1}^N \lambda_i(t) \left( \gamma \left[ M P_i(t) - n_i(t) \right] \right)
\]
where \( \lambda_i(t) \) are the costate variables associated with the dynamic equations for \( n_i(t) \).

\subsubsection{First-Order Conditions}

\begin{enumerate}
    \item For \( \theta_i(t) \):
    \[
    \frac{\partial \mathcal{H}}{\partial \theta_i} = 0
    \]
    
    \item For the costate variables \( \lambda_i(t) \), the costate equations are:
    \[
    \dot{\lambda}_i(t) = \rho \lambda_i(t) - \frac{\partial \mathcal{H}}{\partial n_i}
    \]
\end{enumerate}

\subsubsection{Conclusion}

Solving the dynamic optimization problem involves determining the time path of \( \theta_i(t) \), \( n_i(t) \), and \( \lambda_i(t) \) that satisfies the first-order conditions and boundary conditions. Analytical solutions may be intractable, and numerical methods or approximations may be required.
% @@@@@@@@@@@@@@
